# Supplementary material for: Remember the Past: Distilling Datasets into Addressable Memories for Neural Networks
Source: arXiv:2206.02916 source file (2022-11-19)
Supplement: Supplementary file 2 [file table_cross_arch_appendix.tex]

\begin{wraptable}{r}{6cm}
%\begin{table}[h]
\begin{center}
\begin{tabular}{lcccr}
\toprule
 & ConvNet & AlexNet & ResNet-12 \\
 \hline
ConvNet  & 71.2$\pm$0.4 & 67.5$\pm$0.4 \\
AlexNet  & 65.2$\pm$0.6 & 67.8$\pm$0.3 \\
ResNet12 & 65.2$\pm$0.6 & 67.8$\pm$0.3 \\
 
\bottomrule
\end{tabular}
\end{center}
\caption{Cross architecture generalization.}\label{tbl:cross_arch}
%\end{table}
\end{wraptable}
